# Supplementary material for: Tuning of Magnetic Activity in Spin-Filter Josephson Junctions Towards Spin-Triplet Transport
Source: arXiv:1902.00406 source file (2019-02-01)
Supplement: Supplementary file 1 [file supplementary.pdf]

# Supplementary Material: Tuning of Magnetic Activity in Spin-Filter Josephson Junctions Towards Spin-Triplet transport

## FABRICATION AND EXPERIMENTAL SETUP

The samples presented in this work have been fabricated at the Department of Material Science and Metallurgy of University of Cambridge from NbN-GdN-NbN trilayers grown on oxidized Si substrates using d.c. reactive magnetron sputtering. They have been fabricated in the same fabrication run, by varying GdN thickness by changing the deposition rates, in order to ensure the same deposition conditions for all samples. Different GdN thicknesses do not affect $T_C$ significantly. For GdN thicknesses above 1.5 nm, where the ferromagnetic transition is present, the Curie temperature of GdN, estimated from the $R(T)$ curves as shown in the next Section, remains constant around 35 K (see Fig.1). The junctions have a $7\mu$m $\times$ $7\mu$m mesa geometry defined by optical lithography and selective reactive etching of top NbN layer. A thick Nb layer deposited on top acts as top contact, while the bottom NbN electrode itself acts as bottom contact. NbN layers are 110 nm thick, Nb top electrode is $\approx 400$ nm thick.

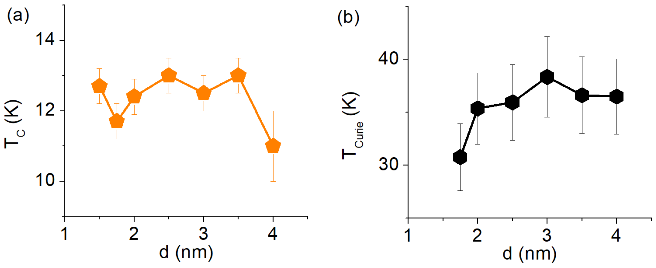


Figure 1. (a) Critical temperature of the junctions as a function of barrier thickness. (b) Curie temperature of the GdN as a function of thickness.

All the measurements presented in this work have been performed using an evaporation cryostat with a base temperature of 0.3 K with customized low noise filters anchored at different temperature stages. The room temperature filters are EMI filters, followed by RC filters anchored to the 1K pot with cut-off frequency of about 1 MHz. Two stages of copper powder filters with cut-off frequencies around 1 GHz are anchored to the 1K pot and to $^3$He pot. Samples are thermally anchored to the $^3$He pot and are current biased, with the voltage collected across the junction using standard four contacts technique. Magnetic field up to 0.3 T in the plane of the junction can be applied using a NbTi coil, which is thermally anchored to the 1K pot of the cryostat[1, 2].

We collect standard $I-V$ characteristics as a function of temperature and magnetic field by biasing the sample with a triangular signal at 11 Hz, and then we extrapolate the critical current using a voltage criterion. We also present measurements of conductance spectra obtained by biasing the sample using a sinusoidal signal at 30 Hz superimposed to a triangular ramp at 1 mHz and measuring the voltage across the junction and the differential conductance via a lock-in amplifier[3].

## SPIN FILTER EFFICIENCY

Spin filter junctions are characterized by a strong supercurrent suppression, compared to standard tunnel junctions with same electrodes and same geometry. The ferromagnetic exchange field $h$ causes the band splitting in GdN, so that spin-up and spin-down electrons see different barrier heights and consequently have different tunneling probabilities. This implies that the tunneling current between the superconducting electrodes is spin polarized, and the barrier acts as a spin filter. The barrier splitting for different spin channels causes the $R(T)$ decrease below the Curie temperature, which is around 35 K (see fig. 2). The spin filter efficiency is defined as [4]

$$P = \frac{|\sigma_\uparrow - \sigma_\downarrow|}{\sigma_\uparrow + \sigma_\downarrow} \quad (1)$$

where $\sigma_\uparrow$ and $\sigma_\downarrow$ are the conductivities for spin up and spin down electrons respectively. Using the WKB approximation for $\sigma$, and assuming that the exchange field $h$ of the ferromagnetic layer is much smaller than the barrier height $E_0$ in absence of exchange field, the spin filter efficiency can be rewritten as[4]

$$P = \tanh\left(\cosh^{-1}\left(\frac{\sigma}{\sigma^*}\right)\right) \quad (2)$$

where $\sigma^*$ is the conductance extrapolated in absence of the exchange field and $\sigma$ is the measured conductance. Both $\sigma$ and $\sigma^*$ can be estimated from experimental $R(T)$ curve (Fig.2), given the general relation $R \propto 1/\sigma$. We define $T_{Curie}$ as the temperature of the maximum of the $R(T)$ curve (green dashed line in Fig. 2). Above this temperature $h = 0$ and $R$ and $R^*$ coincide. For $T < T_{Curie}$, $R^*$ is obtained by extrapolating the fit of $R(T)$ between room temperature and $T_{Curie}$ with a standard semiconducting model.

## MAGNETIC FIELD AND TEMPERATURE BEHAVIOR

Spin filter junctions, as other ferromagnetic junctions featuring a relatively soft ferromagnetic interlayer, are

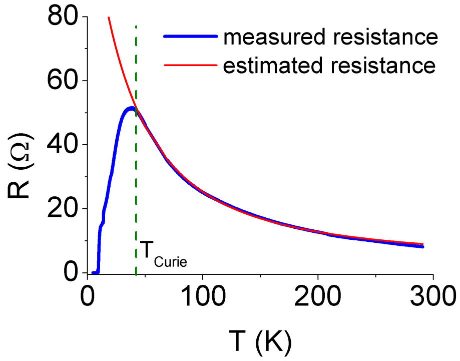


Figure 2. Measured $R(T)$ curve for the sample with 3 nm thick barrier and SFE=0.97 (blue curve), and the extrapolated $R^{*}(T)$ curve in absence of exchange field, obtained by fitting the measured $R(T)$ curve between room temperature and $T_{Curie} \approx 35K$ with a standard semiconducting model.

hysteretic when an external magnetic field is applied, following the magnetization curve of the ferromagnet: when the field is ramped upwards from negative values, the Fraunhofer pattern is shifted towards positive fields, while when the external field is ramped downwards, the $I_C(H)$ curve is shifted towards negative fields, as in Fig. 3 a. These curves present the same features as the ones reported in [5], indicating the presence of a non-conventional current-phase relation.

Following the methods described in [6], it is possible to calculate the $M(H)$ curve from $I_C(H)$ measurements (Fig. 3 b). The results are compatible with the assumption of a relatively soft ferromagnetic barrier with small coercive field ($\approx$ 11 G) and small residual magnetization($\approx$ 300 G). Our findings are also compatible with previous literature on thick unpatterned GdN [7–9].

The presence of a remnant field can significantly change the appearance of $I_C(T)$, and the plateau we observe at intermediate temperatures might be due to residual or trapped magnetic field.

In order to overrule this possibility, we measured $I_C(H)$ curves at different temperatures, and collected their principal maxima, regardless of their position. The temperature dependence of $I_C(H)$ maxima confirms the $I_C(T)$ curves obtained from $I-V(T)$ curves measured before magnetizing the sample and allows us to exclude any effect due to barrier magnetization (Fig.3 c and d).

We have also measured the normal state resistance $R_N$ as a function of temperature for several barrier thicknesses (Fig. 4, left). $R_N$ is roughly constant in the whole temperature range, so $I_C(T)$ and $I_C R_N(T)$ curves are equivalent.

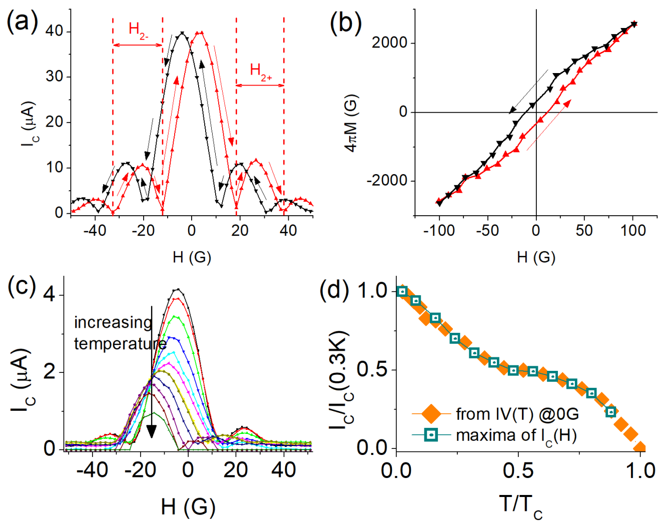


Figure 3. (a) $I_C(H)$ curves at 0.3K for the sample with a 2.5 nm thick barrier. Following Ref.[5], the period of the Fraunhofer pattern is taken as the width $H_{2+} \approx 18.4G$, being $H_{2+}$ the distance between the first two positive minima of the pattern. Arrows indicate the direction of the magnetic field sweeping, and lines are drawn as a guide for the eye. (b) $M(H)$ curve for sample with 2.5 nm thick barrier, calculated from $I_C(H)$ curves following the methods described in [6]. (c) $I_C(H)$ curves at different temperatures for the junction with barrier thickness $d = 3nm$. (d) Comparison between $I_C(T)$ curves obtained from IV characteristics at zero field (orange diamonds) and from the maxima of $I_C(H)$ plot in panel a (dark cyan hollow squares).

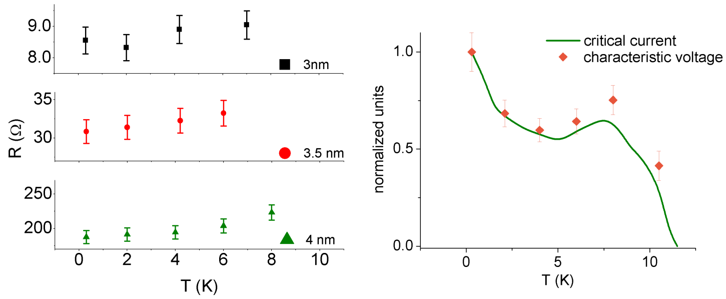


Figure 4. Left: normal state resistance as a function of temperature for different samples. Black squares - 3 nm thick barrier, red circles - 3.5 nm thick barrier, green triangles - 4 nm thick barrier. Right: critical current $I_C$ (green line) and characteristic voltage $I_C R_N$ (orange diamonds) in normalized units as a function of temperature for the sample with 4 nm thick barrier.

## THEORETICAL MODEL

The Andreev levels used to calculate the supercurrent are obtained by solving the following equation[10]:

$$\det \left[ \hat{1} - \hat{r}_{eh}(\epsilon_n)\hat{S}_F^{hh}\hat{r}_{he}(\epsilon_n)\hat{S}_F^{ee} \right] = 0. \qquad (3)$$

$\hat{r}_{eh}$ ($\hat{r}_{he}$) is scattering matrix describing the Andreev reflection process converting an electron (hole) into a hole (electron) at the superconductor-ferromagnet interface. $\hat{S}_F^{ee}(\hat{S}_F^{hh})$ is the scattering matrix describing the electron (hole) propagation in the ferromagnetic layer [11].

The scattering matrix describing the electron (hole) propagation in the ferromagnetic layer can be written as

$$S_F^{ee} = \frac{S_\uparrow + S_\downarrow}{2} \otimes \hat{1} + \frac{S_\uparrow - S_\downarrow}{2} \otimes \hat{\sigma}_z \tag{4}$$

where the matrices $\hat{1}$ and $\hat{\sigma}_z$ are respectively the identity matrix and the z-Pauli matrix acting on the spin space, and the spin dependent scattering matrices are [11]:

$$S_\sigma = e^{i\Theta_\sigma} \begin{pmatrix} \sqrt{1-t_\sigma} & \sqrt{t_\sigma} \\ \sqrt{t_\sigma} & -\sqrt{1-t_\sigma} \end{pmatrix} \tag{5}$$

where $\sigma = \uparrow, \downarrow$ is the electron's spin, $\Theta = \Theta_\uparrow - \Theta_\downarrow$ is the spin mixing angle and $t_\sigma$ is the spin dependent transmission amplitude. The spin mixing angle $0 < \Theta < \pi$ accounts for the spin-dependent scattering phases [12]. The spin filtering is provided by allowing different transparencies for spin up and spin down channels. This model reproduces the Kulik-Omelianchuk limit when $t \sim 1$ and the Ambegaokar Baratoff limit when $t_\uparrow = t_\downarrow << 1$. The different transparencies for spin up and spin down electrodes are modeled as $t_\uparrow = t\cos(\gamma)$ and $t_\downarrow = t\sin(\gamma)$. The angle $\gamma$ varies between 0 and $\pi/4$, and it is derived from the measured spin filter efficiency.

## CONDUCTANCE MEASUREMENTS

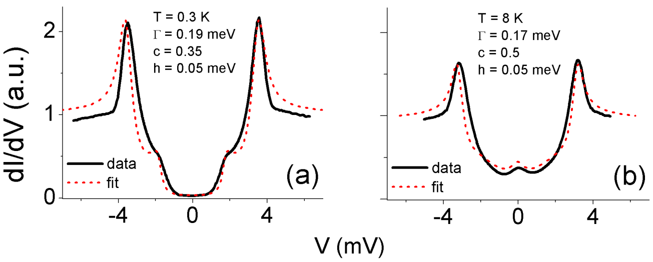


Figure 5. Measured and fitted dI/dV curves for the sample with 3 nm thick barrier, at two different temperatures. T is the temperature, Γ is the broadening, $c$ is the finite background conductance and $h$ is the exchange field. (a) T=0.3 K (b) T=8K.

In Fig.5 we show the experimental data and the fitted curves for the junction with a 3 nm thick barrier at 0.3 K. All measurements have been performed applying a small magnetic field to suppress the Josephson current. The conductance peak corresponding to the sum of the superconducting gap in the two electrodes is at $\approx 3.5$ meV, which is a common value for these spin filter junctions. The peak position follows a typical BCS temperature dependence. The finite background conductance increases as temperature increases, eventually turning into a zero bias peak around 0.7 $T_C$.

The subgap features and the zero bias peak at high temperature observed in all samples can be modeled only if we consider a finite background conductance, which is accounted for adding a phenomenological parameter $c$ in the density of states. This effect is due to the different interfaces between the superconducting electrodes and the barrier. The fitting function used in Fig.5 is obtained combining the results from Meservey et al.[13], Tedrow et al.[14], [15], Dynes et al.[16] and Pal et al.[17]:

$$I \propto a \int_{-\infty}^{+\infty} \rho_1(x+h)\rho_2(x-h+V)\,[f(x)-f(x+V)] + b \int_{-\infty}^{+\infty} \rho_1(x-h)\rho_2(x+h+V)\,[f(x)-f(x+V)] \tag{6}$$

$$\rho = \frac{1}{c+1}\left(\Re\left[\frac{x-\mathrm{i}\Gamma}{\sqrt{(x-\mathrm{i}\Gamma)^2-1}}\right]+c\right) \tag{7}$$

where $a$ and $b$ model the spin filter efficiency, chosen so that $a+b=1$, $h$ is the exchange field of the ferromagnetic barrier, $\Gamma$ is a smearing factor representing the finite lifetime of Cooper pairs [16] and $c$ is a phenomenological term that accounts for the finite background conductance observed in experimental data.

[1] L. Longobardi, D. Massarotti, G. Rotoli, D. Stornaiuolo, G. Papari, A. Kawakami, G. P. Pepe, A. Barone, and F. Tafuri, Appl. Phys. Lett. **99**, 062510 (2011).
[2] D. Massarotti, D. Stornaiuolo, P. Lucignano, L. Galletti, D. Born, G. Rotoli, F. Lombardi, L. Longobardi, A. Tagliacozzo, and F. Tafuri, Phys. Rev. B **92**, 054501 (2015).
[3] D. Stornaiuolo, D. Massarotti, R. Di Capua, P. Lucignano, G. P. Pepe, M. Salluzzo, and F. Tafuri, Phys. Rev. B **95**, 140502 (2017).
[4] K. Senapati, M. G. Blamire, and Z. H. Barber, Nature Materials **10**, 849 (2011).
[5] A. Pal, Z. H. Barber, J. W. A. Robinson, and M. G. Blamire, Nat. Comm. **5**, 3340 (2014).
[6] V. V. Bolginov, V. S. Stolyarov, D. S. Sobanin, A. L. Karpovich, and V. V. Ryazanov, JETP Lett. **95**, 366 (2012).
[7] K. Senapati, T. Fix, M. E. Vickers, M. G. Blamire, and Z. H. Barber, Phys. Rev. B **83**, 014403 (2011).
[8] M. G. Blamire, C. B. Smiet, N. Banerjee, and J. W. A. Robinson, Superconductor Science and Technology **26**, 055017 (2013).
[9] A. Pal, K. Senapati, Z. H. Barber, and M. G. Blamire, Advanced Materials **25**, 5581 (2013).
[10] C. W. J. Beenakker, Phys. Rev. Lett. **67**, 3836 (1991).
[11] T. Tokuyasu, J. A. Sauls, and D. Rainer, Phys. Rev. B **38**, 8823 (1988).
[12] M. Eschrig, Physics Today **64**, 43 (2011).

[13] R. Meservey, P. M. Tedrow, and P. Fulde, Phys. Rev. Lett. **25**, 1270 (1970).
[14] P. M. Tedrow and R. Meservey, Phys. Rev. Lett. **26**, 192 (1971).
[15] P. M. Tedrow, J. E. Tkaczyk, and A. Kumar, Phys. Rev. Lett. **56**, 1746 (1986).
[16] R. C. Dynes, V. Narayanamurti, and J. P. Garno, Phys. Rev. Lett. **41**, 1509 (1978).
[17] A. Pal and M. G. Blamire, Phys. Rev. B **92**, 180510 (2015).
